# Supplementary material for: Three Quantization Regimes for ReLU Networks
Source: arXiv:2405.01952 source file (2024-05-03)
Supplement: Supplementary file 1 [file appendix_general_quantized_weights.tex]

%!TEX root = ../draft_quantized_weight_networks.tex

\section{General weight set $\mathbb{A}$} % (fold)
\label{sec:approximation_error_upper_bounds_of_relu_networks_with_general_quantized_weights_}

	\subsection{Quantization error bound with a general weight set} % (fold)
	\label{sub:quantization_error_bound}

	% \todo{add not necessary finite to the footnote}

	% \todo{ approximation error for general dimension input and weight, and not necessary $finite$, i.e., generalize Proposition~\ref{prop:quantization_error_bound_and_decomposition}.}

	\begin{proposition}
		\label{prop:quantization_error_bound_general}
		Let $d, W,L \in \mathbb{N}$, $B\in \mathbb{R}_+$ such that $B \geq 1$ and $W \geq d$. For all nonempty subsets\footnote{not necessarily finite} $\mathbb{U}, \mathbb{V} \subseteq [-B,B]$, we have
		\begin{equation*}
			\mathcal{A}_\infty ( \mathcal{R}_\mathbb{U} ( ( d,1 ), W,L ), \mathcal{R}_\mathbb{V} ( ( d,1 ), W,L  ) ) \leq L (W+1)^L B^{L-1} \mathcal{A} ( \mathbb{U}, \mathbb{V}, | \cdot |  ).
		\end{equation*} 
		In particular, for all subset\footnote{not necessarily finite} $\mathbb{A} \subset \mathbb{R}$ with $\mathbb{A} \cap [-B,B] \neq \phi$, there holds 
		\begin{align}
			\mathcal{A}_\infty ( \mathcal{R} ( W,L,B  ), \mathcal{R}_\mathbb{A} ( W,L  ) ) \leq&\, L (W+1)^L B^{L-1} \mathcal{A} ( [-B,B], \mathbb{A}\cap [-B,B], | \cdot |  ) \label{eq:quantization_error_bound_general_dimension}\\
			\leq &\, 2 L (W+1)^L B^{L-1} \mathcal{A} ( [-B,B], \mathbb{A}, | \cdot |  ) \label{eq:quantization_error_bound_general_dimension_2}
		\end{align}
	\end{proposition}

	\begin{proof}
		Fix an $\varepsilon > 0$ for now. We note that $\mathcal{A} ( \mathbb{U}, \mathbb{V},| \cdot |  ) = \sup_{u \in \mathbb{U}} \inf_{v \in \mathbb{V}} | u - v |$, and, therefore, for all $u \in \mathbb{U}$ and , we can quantize $u$ into an $v \in \mathbb{V}$, such that the error inccured by the quantization $| u - v | \leq \mathcal{A} (\mathbb{U}, \mathbb{V} ,| \cdot | ) + \varepsilon$. For every $\Phi \in \mathcal{N}_\mathbb{V} ( ( d,1 ), W,L  ) )$, we can apply the same quantization to each weight of $\Phi$ to obtain a network $Q(\Phi) \in \mathcal{N}_\mathbb{V} ( ( d,1 ), W,L  ) )$ with weights in $\mathbb{V}$ such that the resulting absolute difference in each weight is no greater than $\mathcal{A} (\mathbb{U}, \mathbb{V},| \cdot |  ) + \varepsilon$, i.e., 
		\begin{equation}
		\label{_old2_eqline:quantization_minimax_00}
			\| \Phi  - Q ( \Phi ) \| \leq  \mathcal{A} (\mathbb{U}, \mathbb{V} ,| \cdot | ) + \varepsilon,
		\end{equation} with $\| \Phi  - Q ( \Phi ) \|$ defined according to \eqref{eq:weightwise_difference}. We then have 
		\begin{align}
			&\mathcal{A}_\infty ( \mathcal{R}_\mathbb{U} ( ( d,1 ), W,L ), \mathcal{R}_\mathbb{V} ( ( d,1 ), W,L  ) )\label{_old2_eqline:quantization_minimax_0}\\
			 = & \sup_{f \in\mathcal{R}_\mathbb{U} ( ( d,1 ), W,L )} \inf_{\tilde{f} \in\mathcal{R}_\mathbb{V} ( ( d,1 ), W,L  ) } \| f - \tilde{f} \|_{L^\infty ( [0,1]^d )} \label{_old2_eqline:quantization_minimax_10} \\
			= & \sup_{\Phi \in \mathcal{N}_\mathbb{U} ( ( d,1 ), W,L  )} \inf_{\widetilde{\Phi} \in \mathcal{R}_\mathbb{V} ( ( d,1 ), W,L  ) } \| R ( \Phi ) - R ( \widetilde{\Phi} ) \|_{L^\infty ( [0,1]^d )} \\
			\leq & \sup_{\Phi \in \mathcal{N}_\mathbb{U} ( ( d,1 ), W,L  )}  \| R ( \Phi ) - R ( Q ( \Phi )) \|_{L^\infty ( [0,1]^d )} \label{_old2_eqline:quantization_minimax_1}\\
			\leq & \sup_{\Phi \in \mathcal{N}_\mathbb{U} ( ( d,1 ), W,L  )} L (W+1)^L B^{L-1} \| \Phi - Q ( \Phi ) \|\label{_old2_eqline:quantization_minimax_2}\\ 
			\leq &  L (W+1)^L B^{L-1} ( \mathcal{A} (\mathbb{U}, \mathbb{V}  ,| \cdot |) + \varepsilon ),\label{_old2_eqline:quantization_minimax_3}
		\end{align}
		where in \eqref{_old2_eqline:quantization_minimax_1} we used $Q ( \Phi ) \in \mathcal{R}_\mathbb{V} ( ( d,1 ), W,L  )$, for all $\Phi \in \mathcal{N}_\mathbb{U} ( ( d,1 ), W,L  )$, \eqref{_old2_eqline:quantization_minimax_2} follows from Lemma~\ref{lem:quantization_error_general_dimension} with $\Phi^1$ replaced by $ \Phi \in \mathcal{R}_\mathbb{V} ( ( d,1 ), W,L  ) \subseteq \mathcal{R} ( ( d,1 ), W,L, B )$, and $\Phi^2$ replaced by $Q ( \Phi ) \in \mathcal{R}_\mathbb{V} ( ( d,1 ), W,L  ) \subseteq \mathcal{R} ( ( d,1 ), W,L, B )$, and in \eqref{_old2_eqline:quantization_minimax_3} we used \eqref{_old2_eqline:quantization_minimax_00}. Here $\mathcal{R}_\mathbb{V} ( ( d,1 ), W,L  ) \subseteq \mathcal{R} ( ( d,1 ), W,L, B )$ and $\mathcal{R}_\mathbb{V} ( ( d,1 ), W,L  ) \subseteq \mathcal{R} ( ( d,1 ), W,L, B )$ follows from the assumption $\mathbb{U}, \mathbb{V} \subset [-B,B]$. Since \eqref{_old2_eqline:quantization_minimax_0}-\eqref{_old2_eqline:quantization_minimax_3} holds for all $\varepsilon > 0$, we indeed have established
		\begin{equation}
			\label{eq:generl_dimension_B_quantization_error}
			\mathcal{A}_\infty ( \mathcal{R}_\mathbb{U} ( ( d,1 ), W,L ), \mathcal{R}_\mathbb{V} ( ( d,1 ), W,L  ) ) \leq L (W+1)^L B^{L-1} \mathcal{A} (\mathbb{U}, \mathbb{V}  ,| \cdot |) 
		\end{equation}
		as desired. Substituting $\mathbb{U}$ by $[-B,B]$ and $\mathbb{V}$ by $\mathbb{A} \cap [-B,B]$ in \eqref{eq:generl_dimension_B_quantization_error} yields 
		\begin{equation*}
			\mathcal{A}_\infty ( \mathcal{R} ( ( d,1 ), W,L,B ), \mathcal{R}_{\mathbb{A} \cap [-B,B]} ( ( d,1 ), W,L  ) ) \leq L (W+1)^L B^{L-1} \mathcal{A} ([-B,B], \mathbb{A} \cap [-B,B],| \cdot |), 
		\end{equation*}
		which together with $\mathcal{R}_{\mathbb{A} \cap [-B,B]} ( ( d,1 ), W,L  ) \subseteq \mathcal{R}_{\mathbb{A} } ( ( d,1 ), W,L  )$ establishes \eqref{eq:quantization_error_bound_general_dimension}. Then \eqref{eq:quantization_error_bound_general_dimension_2} follows from combing \eqref{eq:quantization_error_bound_general_dimension} and the relation
		\begin{equation*}
		 	\mathcal{A} ([-B,B], \mathbb{A} \cap [-B,B],| \cdot |) \leq 2 \mathcal{A} ([-B,B], \mathbb{A},| \cdot |)
		\end{equation*} 
		provided by a technical result Lemma~\ref{lem:auxiliary_lemma_minimax_r} in Appendix~\ref{lem:auxiliary_lemma_minimax_r}.
	\end{proof}
