# Supplementary material for: Three Quantization Regimes for ReLU Networks
Source: arXiv:2405.01952 source file (2024-05-03)
Supplement: Supplementary file 2 [file appendix_general_tradeoff.tex]

%!TEX root = ../draft_quantized_weight_networks.tex


	% \subsection{General weight tradeoff approximation} % (fold)
	% \label{sub:general_weight_tradeoff_approximation}
	% \todo{Use only the approximation form rather than the density form.}
	% % subsection general_weight_tradeoff_approximation (end)

	% \todo{Start by recalling the quantization error bound given in \eqref{eq:error_decomposition_binary_quantized_weights}}
	% \todo{We asking the same problems, if the precision is correct then how do we trade off? }

	% \todo{Give the density results.}


	% Recall that in \label{eq:error_decomposition_general_quantized_weights} Section~\ref{sec:bounds_on_quantization_error}, we obtain an upper bound on $\mathcal{A}_\infty ( \lip  ( [0,1] ), \mathcal{R}_\mathbb{A} (W, L  )  )$, ????,  according to
	% \begin{align*}
	% 	\mathcal{A}_\infty ( \lip  ( [0,1] ), \mathcal{R}_\mathbb{A} (W, L  )  )  \leq&\,   C  ( W^2 L^2 \log (W)  )^{-1}  + L (W+1)^L \mathcal{A} ( [-1,1], \mathbb{A}\cap [-1,1], | \cdot |  )\\
	% 	\leq &\, C  ( W^2 L^2 \log (W)  )^{-1}  + 2 L (W+1)^L \mathcal{A} ( [-1,1], \mathbb{A}, | \cdot |  ).
	% \end{align*}
	% If the weight set $\mathbb{A}$ is of high precision, in the sense of a small $\mathcal{A} ( [-1,1], \mathbb{A}\cap [-1,1], | \cdot |  ) $ and $\mathcal{A} ( [-1,1], \mathbb{A}, | \cdot |  )$, such that the upper bound on error incurred by quantization $2 L (W+1)^L \mathcal{A} ( [-1,1], \mathbb{A}, | \cdot |  )$ is of the order $ W^2 L^2 \log (W) $, the overall apprximation error $\mathcal{A}_\infty ( \lip  ( [0,1] ), \mathcal{R}_\mathbb{A} (W, L  )  )$ is at most of the order $ W^2 L^2 \log (W) $. If the precision the precision of $\mathbb{A}$ is not enough, we show in Sec~?? in the case of binary quantized weight with $\mathbb{A} = \mathbb{Q}_b^a$ for some $a,b \in \mathbb{N}$, we can trade depth for a higher precision. We now show that, the same tradeoff also holds for a general weight set $\mathbb{A}$. \todo{ a different story??}

	% \todo{Start from the triangle inequality.}

	% \begin{equation}
	% \label{eq:quantization_error_bound_general_dimension}
	% 	\mathcal{A}_\infty ( \mathcal{R} ( W,L,B  ), \mathcal{R}_\mathbb{A} ( W,L  ) ) \leq 2 L (W+1)^L B^{L-1} \mathcal{A} ( [-B,B], \mathbb{A}, | \cdot |  ).
	% \end{equation}




	% The main theorem is as follows.



	

	% \begin{proposition}
	% 	% \label{prop:quantization_error_bound_and_decomposition}
	% 	Let $W,L \in \mathbb{N}, k$, $B\in \mathbb{R}_+$ with $B \geq 1$. For all subset $\mathbb{A} \subset \mathbb{R}$, there holds 
	% 	\begin{equation*}
	% 		\begin{aligned}
	% 			\mathcal{A}_\infty ( \mathcal{R} ( W,L,B  ), \mathcal{R}_\mathbb{A} ( 16W,(k+2) L  ) ) \leq L (W+1)^L B^{L-1} (2  \mathcal{A} ( [- ( B^{1\slash k} + 1 ),B^{1\slash k} + 1], \mathbb{A}, | \cdot |  ) )^k.
	% 		\end{aligned}
	% 	\end{equation*}
	% \end{proposition}


	% \todo{Comparing the results to existence results}
	% \vspace{10em}

	% \todo{we proceed to the proof of ?? }

	% Recall that for all ???, we have 
	% \begin{equation*}
	% 	\mathcal{R}_{\mathcal{T}_1 ( \mathbb{A},u,v,k)} (( d,d' ),  W,  L  ) \subseteq  \mathcal{R}_\mathbb{A} ( ( d,d' ), 16W,(k+3) L )
	% \end{equation*}
	% with
	% \begin{equation}
	% 		% \label{eq:def_Auvk_new}
	% 	\mathcal{T}_1 ( \mathbb{A},u,v,k) := \biggl\{ \sum_{i = 0}^{k} (u^i a_i + v^i b_i) : | a_i |,| b_i | \in \mathbb{A} , i = 0,\dots, k \biggr\}.	
	% \end{equation}
	% We already have
	% \begin{align}
	% % \label{eq:quantization_error_bound_general_dimension}
	% 	&\,\mathcal{A}_\infty ( \mathcal{R} ( ( d,d' ),W,L,B  ), \mathcal{R}_\mathbb{A} ( ( d,d' ),16W,( k+3 )L  ) ) \\
	% 	\leq &\, \mathcal{A}_\infty ( \mathcal{R} ( ( d,d' ),W,L,B  ), \mathcal{R}_{\mathcal{T}_1 ( \mathbb{A},u,v,k)} ( ( d,d' ),W,L  ) ) \\
	% 	\leq&\, 2 L (W+1)^L B^{L-1} \mathcal{A} ( [-B,B], {\mathcal{T}_1 ( \mathbb{A},u,v,k)}, | \cdot |  ).
	% \end{align}

	% Therefore, it suffice to show that

	% \begin{equation*}
	% 	\mathcal{A} ( [-B,B], {\mathcal{T}_1 ( \mathbb{A},u,v,k)}, | \cdot |  ) \leq (  \mathcal{A} ( [- ( B^{1\slash k} + 1 ),B^{1\slash k} + 1], \mathbb{A}, | \cdot |  ) )^k  ,
	% \end{equation*}

	%  which is establishes as follows.

	% \begin{enumerate}
	% 	\item What if $\mathbb{A}$ cannot approximate $B$ from both side? 
	% \end{enumerate}

	

	% \vspace{10em}

	% \begin{proposition}
	% Suppose $\{ -1,0,1 \} \subseteq \mathbb{A}$, and
	% \begin{equation*}
	% 	\mathcal{A} ( [-(B +1) ,B + 1], \mathbb{A}, | \cdot | ) \leq 1,
	% \end{equation*}
	% then we have
	% \begin{align*}
	% 	\inf_{u,v \in \mathbb{A}} \mathcal{A} ( [-B^k,B^k], \mathcal{T}_1 ( \mathbb{A},u,v,k), | \cdot | ) \leq  2^{k-1} ( \mathcal{A} ( [-(B +1) ,B + 1], \mathbb{A}, | \cdot | ) )^k,
	% \end{align*}
	% with $\mathcal{T}_1 ( \mathbb{A},u,v,k), | \cdot | )$ given in \eqref{eq:def_Auvk_new}. 
	% \end{proposition}

	% \begin{proof}
	% 	Suppose first that $\mathbb{A}$ is closed. We shall show the existence of $u,v$ such that, for all $x \in [-B^k, B^k] $, there exists an $y \in \mathcal{T}_1 ( \mathbb{A},u,v,k)$ such that 
	% 	\begin{equation*}
	% 		| x - y  | \leq ( \mathcal{A} ( [-(B +1) ,B + 1], \mathbb{A}, | \cdot | ) )^k.
	% 	\end{equation*}

	% 	We will use an Euclidean type algorithm to determine $y$, and the ingredient is as follows.

	% 	For simplexity of the notation, we note
	% 	\begin{equation*}
	% 		\varepsilon =  \mathcal{A} ( [-(B +1) ,B + 1], \mathbb{A}, | \cdot | ).
	% 	\end{equation*}

	% 	\begin{enumerate}
	% 		\item For all $x \in [-B,B]$, there exists a real number $a$ with $| a | \in \mathbb{A} $ such that 
	% 		\begin{equation}
	% 		\label{eq:algorithm_condition_1}
	% 			| a - x | \leq \varepsilon. 
	% 		\end{equation}

	% 		\item There exist a real number $u \in \mathbb{A}$ such that 
	% 		\begin{equation}
	% 		\label{eq:algorithm_condition_2}
	% 			u \geq B. 
	% 		\end{equation}

	% 		\item There exist a real number $v \in \mathbb{A}$ such that 
	% 		\begin{equation}
	% 		\label{eq:algorithm_condition_3}
	% 			v \leq 2 \varepsilon.
	% 		\end{equation}
	% 	\end{enumerate}

	% 	Specifically, we shall show the existence of $\sum_{i = 0}^{k} (u^i a_i + v^i b_i) \Bigr| = \Bigl| y - \sum_{i = 0}^{k} (v^i b_i) \in  \mathcal{T}_1 ( \mathbb{A},u,v,k)$ such that 
	% 	\begin{equation*}
	% 		| x - \sum_{i = 0}^{k} (u^i a_i + v^i b_i) | = \Bigl| y - \sum_{i = 0}^{k} (v^i b_i) |  \leq 2^k \varepsilon.
	% 	\end{equation*}


	% 	\todo{Define the set $\{ a: | a | \in \mathbb{A}  \}$}

	% 	The algorithm consists of two parts, in sequence. The first part concerns the determination of $( a_i )_{i =0}^{k}$ such that $| a_i | \in \mathbb{A} $, $| x - \sum_{i = 0}^{k} (u^i a_i + v^i b_i) | \leq \varespilon$ and is effected by $k + 1$ step, such that in the $j$-th step, $j = 1,\dots, k+ 1$, we determined $( a_i )_{i =k + 1 -j}^{k }$ such that 
	% 	\begin{equation*}
	% 		| x - \sum_{i = k + 1 -j}^{k} (u^i a_i + v^i b_i) | \leq u^{k-j} \varepsilon.
	% 	\end{equation*}

	% 	The algorithm is given as follows in a form of induction. 

	% 	For $j = 1$, the first step is as follows. We note that $ x \in [-B^k,B^k]$ implies $| \frac{x}{u^{k-1}} | \leq  | \frac{x}{B^{k-1}} | \leq B$. Then it follows from Property $1$ the existence of $a_{k-1}$ such that $| \frac{x}{v^{k-1}} - a_{k-1}| \leq \varepsilon $, which is yields 
	% 	\begin{equation*}
	% 		|x - a_{k-1} {v^{k-1}}| \leq {v^{k-1}} \varepsilon 
	% 	\end{equation*}
	% 	as desired. Suppose we have obtain an sequence of 
		
	% \end{proof}
		
	

	












	% \vspace{10em}
	% \begin{proposition}
	% 	% \label{thm:general_representation}
	% 	Let $d,d',W,L \in \mathbb{N}$, and $\mathbb{A} \subseteq \mathbb{R}$ with $\{ -1,0,1 \} \subseteq \mathbb{A}$. Then for every $k \in \mathbb{N}$ and all $u,v \in \mathbb{A} \cap \mathbb{R}_{\geq 0}$, there holds
	% 	\begin{equation*}
	% 		\mathcal{R}_{\mathcal{T}_1 ( \mathbb{A},u,v,k)} (( d,d' ),  W,  L  ) \subseteq  \mathcal{R}_\mathbb{A} ( ( d,d' ), 16W,(k+3) L )
	% 	\end{equation*}
	% 	with
	% 	\begin{equation}
	% 		\label{eq:def_Auvk_new}
	% 		\mathcal{T}_1 ( \mathbb{A},u,v,k) := \biggl\{ \sum_{i = 0}^{k} (u^i a_i + v^i b_i) : | a_i |,| b_i | \in \mathbb{A} , i = 0,\dots, k \biggr\}.	
	% 	\end{equation} 
	% \end{proposition}


	% \begin{proposition}
	% 	\begin{align*}
	% 		\inf_{u,v \in \mathbb{A}} \mathcal{A} ( [-B,B], [-B,B]\cap \mathcal{T}_1 ( \mathbb{A},u,v,k), | \cdot | ) \leq  ( 8\mathcal{A} ( [0,B^{1\slash k} + 1], [0,B^{1\slash k} + 1]\cap \mathbb{A}, | \cdot | ) )^k,
	% 	\end{align*}
	% 	with $\mathcal{T}_1 ( \mathbb{A},u,v,k), | \cdot | )$ given in \eqref{eq:def_Auvk_new}. 
	% \end{proposition}



	

	


	% \subsection{proof of ??? } % (fold)
	% \label{sub:proof_of_}
	
	% % subsection proof_of_ (end)

	% \begin{proposition}
	% 	Let 
	% \end{proposition}

	% \vspace{4em}
	% Recall that ??? The proof needs the representation
	



	% \begin{proposition}
	% 	% \label{prop:quantization_error_bound_and_decomposition}
	% 	Let $W,L \in \mathbb{N}$, $B\in \mathbb{R}_+$ with $B \geq 1$. For all finite subset $\mathbb{A} \subset \mathbb{R}$, there holds 
	% 	\begin{equation*}
	% 		\mathcal{A}_\infty ( \mathcal{R} ( W,L,B  ), \mathcal{R}_\mathbb{A} ( W,L  ) ) \leq L (W+1)^L B^{L-1} \mathcal{A} ( [-B,B], \mathbb{A}\cap [-B,B], | \cdot |  ).
	% 	\end{equation*}
	% 	% In particular, for all $a,b \in \mathbb{N}$ such that $B \leq 2^a$, there hold $\mathcal{A} ( [-B,B], \mathbb{Q}_b^a\cap [-B,B], | \cdot | ) \leq 2^{-b}$, and 
	% 	% \begin{equation}
	% 	% 	\label{eq:quantization_binary_A}
	% 	% 	\mathcal{A}_\infty ( \mathcal{R} ( W,L,B  ), \mathcal{R}_b^a ( W,L  ) ) \leq L (W+1)^L B^{L-1} 2^{-b}.
	% 	% \end{equation}
	% \end{proposition}




	% % \todo{Another ingredients is ???}.
	% \begin{proposition}
	% 	\begin{align*}
	% 		\inf_{u,v \in \mathbb{A}} \mathcal{A} ( [-B,B], [-B,B]\cap \mathcal{T}_1 ( \mathbb{A},u,v,k), | \cdot | ) \leq  ( 8\mathcal{A} ( [0,B^{1\slash k} + 1], [0,B^{1\slash k} + 1]\cap \mathbb{A}, | \cdot | ) )^k,
	% 	\end{align*}
	% 	with $\mathcal{T}_1 ( \mathbb{A},u,v,k)$ given in \eqref{eq:def_Auvk_new}. 
	% \end{proposition}


	% \begin{proof}
	% 	Since $\mathbb{A}$ is $\varepsilon$-dense in $[-B,B]$, there exists $u,v\in \mathbb{A} \cap [-B,B]$ such that $| v - 2 \varepsilon | \leq \varepsilon $ and $| u- B | \leq \varepsilon$, which implies
	% 	\begin{align*}
	% 		u \in& [B - \varepsilon, B]\\
	% 		v \in& [\varepsilon, 3\varepsilon]			
	% 	\end{align*}
	% 	It remains to show that $\mathbb{A}(u,v,k)$ is $(3\varepsilon)^{k}$ dense in $[-(B- \varepsilon)^k, (B- \varepsilon)^k]$. We fix an $x \in [(B- \varepsilon)^{k+1},(B- \varepsilon)^{k}] $ and use the Euclidean algorithm, as follows, to find $( a_i )_{i=0}^k$ and $( b_i )_{i=0}^k$ such that  $| x - \sum_{i = 0}^{k} (u^i a_i + v^i b_i) | \leq v^k \varepsilon \leq (3 \varepsilon)^{k+1}$ and $| a_i |,| b_i | \in \mathbb{A} $, $i =0,\dots,k$. Since $ 0 \leq | \frac{x}{v^{k}} |  \leq  | \frac{(B-\varepsilon)^{k+1}}{(B- \varepsilon)^{k}}  |  \leq B$, and $\mathbb{A}$ is $\varepsilon$-dense on $[-B,B]$,  there exists a number $\tilde{a}_k \in A \cap [-B,B]$ such that 
	% 	\begin{equation}
	% 		\label{eq:choice_of_tilde_a_k}
	% 	 	\biggl|\tilde{a}_k -  \biggl| \frac{x}{u^{k}}  \biggr|  \biggr| \leq \varepsilon.
	% 	\end{equation} 
	% 	Set $a_k = \tilde{a}_k $, if $x \geq 0$, and $a_k = - \tilde{a}_k $, otherwise. It then follows from \eqref{eq:choice_of_tilde_a_k} that  $|a_k -  \frac{x}{u^{k}}   | \leq \varepsilon$, which implies $|\frac{x - a_k u^k}{u^{k-1}}   | \leq u \varepsilon  \leq B$. Since $\tilde{a}_k \in \mathbb{A}$ and $\mathbb{A} = -\mathbb{A}$, we have $| a_k | \in \mathbb{A} $. We continue to find $a_{k-1}$. Since $| \frac{x - a_k u^k  }{u^{k-1}}| \leq B $ and by a similar way we can find an $a_{k-1}$ with $| a_{k-1} |\in \mathbb{A} $ such that $| \frac{x - a_k u^k  }{u^{k-1}} - a_{k-1} | \leq \varepsilon$, which implies $| \frac{x - a_k u^k - a_{k-1}u^{k-1} }{u^{k-2}} | \leq u \varepsilon \leq B$. Repeating the same algorithm yields the existence of  $a_i$ with $| a_i |\in \mathbb{A}$, $i = 0,\dots, k $ such that $| \frac{x - \sum_{i =0}^k a_k u^k}{u^{-1}} | \leq u \varepsilon$, which implies  $| x - \sum_{i =0}^k a_k u^k | \leq \varepsilon$. We set $y =  x - \sum_{i =0}^k a_k u^k$ and implement the Euclidean algorithm on $y$ with respect to $v$. Since $| y | \leq \varepsilon \leq B$, with a similar argument, when searching for $a_k$, there exist $b_0 \in \mathbb{R}$ such that $| b_0 | \in \mathbb{A}$ and $| y - b_0 | \leq \varepsilon$. We then get $| \frac{y - b_0}{v} | \leq  \frac{\varepsilon}{v} \leq 1 \leq B$, and, in turn, the existence of $b_1$  such that $| b_1 | \in \mathbb{A}$ and $| \frac{y - b_0}{v} - b_1  |\leq \varepsilon$, which in turn implies $| \frac{y - b_0 - b_1 v}{v^2} |\leq \frac{\varepsilon}{v} \leq B$. Repeating the same algorithm, yields the existence of $b_i \in \mathbb{R}_+$ with $| b_i  | \in \mathbb{A}$, $i =0,\dots,k$ such that  $| \frac{y - \sum_{i=0}^k v^i b_i}{v^{k+1}} | \leq \frac{\varepsilon}{v} $, which is $y - \sum_{i=0}^k v^i b_i \leq v^k \varepsilon$. It follows that
	% 	\begin{equation*}
	% 		\Bigl| x - \sum_{i = 0}^{k} (u^i a_i + v^i b_i) \Bigr| = \Bigl| y - \sum_{i = 0}^{k} (v^i b_i) \Bigr| \leq v^k \varepsilon \leq (3 \varepsilon)^{k+1},
	% 	\end{equation*}
	% 	where we used $v \leq 3 \varepsilon$, and therefore we find an element $y = \sum_{i = 0}^{k} (u^i a_i + v^i b_i)$ such that $| x - y | \leq  (3 \varepsilon)^{k+1}$. This procedure holds for all $x \in [-(B - \varepsilon)^{k+1}, (B+\varepsilon)^{k+1}]$ and therefore $\mathbb{A}(u,v,k)$ is $(3 \varepsilon)^{k} \varepsilon$-dense in $[- (B - \varepsilon)^{k+1}, (B - \varepsilon)^{k+1}]$. 
	% \end{proof}


	% \vspace{10em}
	% Since $\mathbb{A}$ is $\varepsilon$-dense in $[-B,B]$, there exists $u,v\in \mathbb{A} \cap [-B,B]$ such that $| v - 2 \varepsilon | \leq \varepsilon $ and $| u- B | \leq \varepsilon$, which implies
	% \begin{align*}
	% 	u \in& [B - \varepsilon, B]\\
	% 	v \in& [\varepsilon, 3\varepsilon]			
	% \end{align*}
	% It remains to show that $\mathbb{A}(u,v,k)$ is $(3\varepsilon)^{k}$ dense in $[-(B- \varepsilon)^k, (B- \varepsilon)^k]$. We fix an $x \in [(B- \varepsilon)^{k+1},(B- \varepsilon)^{k}] $ and use the Euclidean algorithm, as follows, to find $( a_i )_{i=0}^k$ and $( b_i )_{i=0}^k$ such that  $| x - \sum_{i = 0}^{k} (u^i a_i + v^i b_i) | \leq v^k \varepsilon \leq (3 \varepsilon)^{k+1}$ and $| a_i |,| b_i | \in \mathbb{A} $, $i =0,\dots,k$. Since $ 0 \leq | \frac{x}{v^{k}} |  \leq  | \frac{(B-\varepsilon)^{k+1}}{(B- \varepsilon)^{k}}  |  \leq B$, and $\mathbb{A}$ is $\varepsilon$-dense on $[-B,B]$,  there exists a number $\tilde{a}_k \in A \cap [-B,B]$ such that 
	% \begin{equation}
	% 	\label{eq:choice_of_tilde_a_k}
	%  	\biggl|\tilde{a}_k -  \biggl| \frac{x}{u^{k}}  \biggr|  \biggr| \leq \varepsilon.
	% \end{equation} 
	% Set $a_k = \tilde{a}_k $, if $x \geq 0$, and $a_k = - \tilde{a}_k $, otherwise. It then follows from \eqref{eq:choice_of_tilde_a_k} that  $|a_k -  \frac{x}{u^{k}}   | \leq \varepsilon$, which implies $|\frac{x - a_k u^k}{u^{k-1}}   | \leq u \varepsilon  \leq B$. Since $\tilde{a}_k \in \mathbb{A}$ and $\mathbb{A} = -\mathbb{A}$, we have $| a_k | \in \mathbb{A} $. We continue to find $a_{k-1}$. Since $| \frac{x - a_k u^k  }{u^{k-1}}| \leq B $ and by a similar way we can find an $a_{k-1}$ with $| a_{k-1} |\in \mathbb{A} $ such that $| \frac{x - a_k u^k  }{u^{k-1}} - a_{k-1} | \leq \varepsilon$, which implies $| \frac{x - a_k u^k - a_{k-1}u^{k-1} }{u^{k-2}} | \leq u \varepsilon \leq B$. Repeating the same algorithm yields the existence of  $a_i$ with $| a_i |\in \mathbb{A}$, $i = 0,\dots, k $ such that $| \frac{x - \sum_{i =0}^k a_k u^k}{u^{-1}} | \leq u \varepsilon$, which implies  $| x - \sum_{i =0}^k a_k u^k | \leq \varepsilon$. We set $y =  x - \sum_{i =0}^k a_k u^k$ and implement the Euclidean algorithm on $y$ with respect to $v$. Since $| y | \leq \varepsilon \leq B$, with a similar argument, when searching for $a_k$, there exist $b_0 \in \mathbb{R}$ such that $| b_0 | \in \mathbb{A}$ and $| y - b_0 | \leq \varepsilon$. We then get $| \frac{y - b_0}{v} | \leq  \frac{\varepsilon}{v} \leq 1 \leq B$, and, in turn, the existence of $b_1$  such that $| b_1 | \in \mathbb{A}$ and $| \frac{y - b_0}{v} - b_1  |\leq \varepsilon$, which in turn implies $| \frac{y - b_0 - b_1 v}{v^2} |\leq \frac{\varepsilon}{v} \leq B$. Repeating the same algorithm, yields the existence of $b_i \in \mathbb{R}_+$ with $| b_i  | \in \mathbb{A}$, $i =0,\dots,k$ such that  $| \frac{y - \sum_{i=0}^k v^i b_i}{v^{k+1}} | \leq \frac{\varepsilon}{v} $, which is $y - \sum_{i=0}^k v^i b_i \leq v^k \varepsilon$. It follows that
	% \begin{equation*}
	% 	\Bigl| x - \sum_{i = 0}^{k} (u^i a_i + v^i b_i) \Bigr| = \Bigl| y - \sum_{i = 0}^{k} (v^i b_i) \Bigr| \leq v^k \varepsilon \leq (3 \varepsilon)^{k+1},
	% \end{equation*}
	% where we used $v \leq 3 \varepsilon$, and therefore we find an element $y = \sum_{i = 0}^{k} (u^i a_i + v^i b_i)$ such that $| x - y | \leq  (3 \varepsilon)^{k+1}$. This procedure holds for all $x \in [-(B - \varepsilon)^{k+1}, (B+\varepsilon)^{k+1}]$ and therefore $\mathbb{A}(u,v,k)$ is $(3 \varepsilon)^{k} \varepsilon$-dense in $[- (B - \varepsilon)^{k+1}, (B - \varepsilon)^{k+1}]$. 


	\iffalse

	\subsection{General results???} % (fold)
	\label{sub:general_results_}
	
	% subsection general_results_ (end)

		\todo{General weight set formulation??}


		\rmk{tradeoff}
		\begin{proposition}
			More generally, for all $E, B,\varepsilon \in \mathbb{R}_+$, finite subset $\mathbb{A} \subseteq \mathbb{R} $ such that $\varepsilon < 1\slash 2$, $ 1 \leq B \leq  (E - \varepsilon)^{k}$, and  $\mathbb{A}$ is $\varepsilon$-dense in $[-E,E]$ with $\{ -1,0,1 \} \subseteq \mathbb{A}$, $\mathbb{A} = -\mathbb{A} := \{ -x: x \in \mathbb{A} \}$, we have
			\begin{equation}
			% \label{eq:approximation_error_general_weights}
			\begin{aligned}
				 &\mathcal{A}_\infty \left( \mathcal{R} \left( d,W,L, B \right), \mathcal{R}_\mathbb{A} \left( d, 16W,(k+2) L\right) \right) \\
				 \leq & \,  L \left( W+1 \right)^L B^{L-1} (3 \varepsilon)^{k}.
			\end{aligned}
			\end{equation}
			\begin{proof}
				See Appendix~\ref{sec:approximation_error_upper_bounds_of_relu_networks_with_general_quantized_weights_}.
			\end{proof}
		\end{proposition}

		\rmk{$\epsilon$-dense}
		\begin{definition}
			[$\varepsilon$-denseness] Suppose $B \in [-B,B]$. A finite set $\mathbb{A} \subseteq \mathbb{R}$ is said to be $\varepsilon$-dense in $[-B,B]$ if 
			% $\mathcal{A} ( [-B,B], \mathbb{A} \cap [-B,B], | \cdot |  ) \leq \varepsilon$, i.e.  
			for every number $x \in [-B,B]$, there exists a number $y \in \mathbb{A} \cap [-B,B]$ such that $| x - y | \leq \varepsilon$.
			\label{def:epsilon_dense}
		\end{definition}



		The second part of the proof regarding general weight sets will require two more following lemmas in addition to Lemma~\ref{thm:general_representation}.

		% \begin{align}
		% 	&\mathcal{R}^{ka}_{kb} (d,  W,  L) \\
		% 	=& \mathcal{R} (d,  W,  L, \mathbb{Q}_{kb}^{ka}  )\\
		% 	\subseteq & \mathcal{R}_{\mathbb{A}(u,v,k-1)} (d,  W,  L  ) \label{eqline:using_inclusion}\\
		% 	\subset&  \mathcal{R} ( d, 16W,(k+2) L, \mathbb{Q}_b^a )\label{eqline:applying_representation_theorem} \\
		% 	=& \mathcal{R}_b^a (d,16W,(k+2)L).
		% \end{align}
		% where \eqref{eqline:using_inclusion} used the inclusion relation \eqref{eq:inclusion}, and \eqref{eqline:applying_representation_theorem} used Lemma~\ref{thm:general_representation}.

		


	



	\begin{lemma}
		\label{lem:density}
		Suppose $B,\varepsilon \in \mathbb{R}_+$ with $B \geq 1$ and $\varepsilon < 1\slash 2$, $k \in \mathbb{N}$, and $\mathbb{A} \subseteq \mathbb{R}$ is $\varepsilon$-dense in $[-B,B]$. Then there exists $u,v \in \mathbb{A} \cap \mathbb{R}_{\geq 0}$ such that 
		\begin{equation}
			\mathbb{A}(u,v,k) := \{ \sum_{i = 0}^{k} (u^i a_i + v^i b_i) : | a_i |, | b_i | \in \mathbb{A} , i = 0,\dots, k \} 	
		\end{equation} 
		is$(3\varepsilon)^{k} \varepsilon$-dense in $[(B- \varepsilon)^{k+1} , (B- \varepsilon)^{k+1}] $ with $\mathbb{A} = -\mathbb{A}$. 
	\end{lemma}
	\begin{lemma}
		\label{lem:density_transfer}
		Suppose that $B,C , \varepsilon\in \mathbb{R}_+$ such that $ B \geq C > \varepsilon$, set $\mathbb{A}$ is $\varepsilon$-dense in $[-B,B]$. Then $\mathbb{A}$ is $2 \varepsilon$-dense in $[-C,C]$ 
	\end{lemma}
	The proof of these two lemmas are deferred until Appendix~\ref{sub:density_of_the_set_} and Appendix~\ref{sub:density_on_a_subset}, respectively, and we proceed to the remaining proof of the proposition. Let $E,B,\varepsilon \in \mathbb{R}_+$, and $\mathbb{A} \subset \mathbb{R}$ be a finite set that is $\varepsilon$-dense in $[-E,E]$ with $\{ -1,0,1 \} \subseteq \mathbb{A}$ such that $1 \leq B \leq (E- \varepsilon)^k$. Suppose firstly that $k =1$. As $\mathcal{R}_\mathbb{A} ( d, W,L )  \subseteq \mathcal{R}_\mathbb{A} ( d, 16W,(k+2) L ) $, we get 
	\begin{align}
		&\mathcal{A}_\infty ( \mathcal{R} ( d,W,L, B ), \mathcal{R} ( d, 16W,(k+2) L) )\\
		\leq& \mathcal{A}_\infty ( \mathcal{R} ( d,W,L, B ), \mathcal{R}_\mathbb{A} ( d, W,L) )\\
		\leq & L ( W+1 )^L B^{L-1} 2 \varepsilon \label{eqline:applying_tradeoff_realization_1}
	\end{align}
	where in \eqref{eqline:applying_tradeoff_realization_1} we applied Proposition~\ref{prop:quantization_error_bound_and_decomposition} together with $\mathbb{A}$ being $2 \varepsilon$-dense in $[-B,B]$, that follows from Lemma~\ref{lem:density_transfer}.
		%  $\mathbb{A}$ is $2 \varepsilon$-dense on the subset $[-B,B]$
		% Since $\mathbb{A}$ is $2 \varepsilon$-dense in $[- (E - \varepsilon), E - \varepsilon]$, according to Lemma~\ref{lem:density_transfer}, $\mathbb{A}$ is $2 \varepsilon$-dense on the subset $[-B,B]$. Then it follows from Proposition~\ref{prop:quantization_error_bound_and_decomposition} that 
		% \begin{align*}
		% 	\mathcal{A}_\infty ( \mathcal{R} ( d,W,L, B ), \mathcal{R} ( d, W,L) ) \leq&  L ( W+1 )^L B^{L-1} 2 \varepsilon\\
		% 	\leq & L ( W+1 )^L B^{L-1} 3 \varepsilon.
		% \end{align*}
	Suppose otherwise that $k \geq 2$. Lemma~\ref{lem:density} implies the existence of $u,v \in \mathbb{A} \cap \mathbb{R}_{\geq 0}$ such that $\mathbb{A}(u,v,k -1 )$ is $(3 \varepsilon)^{k-1} \varepsilon $-dense in $[-(E- \varepsilon)^k, (E - \varepsilon)^k]$, and, in consequence, $2 (3 \varepsilon)^{k-1}\varepsilon$-dense in $[-(B- \varepsilon)^k, (B - \varepsilon)^k]$ by Lemma~\ref{lem:density_transfer}. Then it follows from Lemma~\ref{thm:general_representation} that 
	\begin{equation}
		\label{eq:embedding_general_weights}
		\mathcal{R}_{\mathbb{A}(u,v,k -1 )} (d,  W,  L  ) \subseteq \mathcal{R}_\mathbb{A} ( d, 16W,(k+2) L) ,
	\end{equation}
	We get
	\begin{align}
		&\mathcal{A}_\infty ( \mathcal{R}_\mathbb{A} ( d,W,L ), \mathcal{R} ( d, 16W,(k+2) L) )\\
		\leq& \mathcal{A}_\infty ( \mathcal{R} ( d,W,L, B ), \mathcal{R}_{\mathbb{A}(u,v,k -1 )} (d,  W,  L  ) ) \label{eqline:embedding_general_weights_1} \\
		\leq &\, L ( W+1 )^L B^{L-1} 2 (3 \varepsilon)^{k-1} \varepsilon  \label{eqline:embedding_general_weights_2}\\
		\leq &\,  L ( W+1 )^L B^{L-1} (3 \varepsilon)^{k}
	\end{align}
	where \eqref{eq:embedding_general_weights} follows from \eqref{eqline:embedding_general_weights_2}, and in we apply Proposition~\ref{prop:quantization_error_bound_and_decomposition} with $\mathbb{A}$ $2 (3 \varepsilon)^{k-1} \varepsilon$-dense in $[-(B- \varepsilon)^k, (B - \varepsilon)^k]$.



	



	% \subsection{Proof of Lemma~\ref{lem:density}} % (fold)
	% \label{sub:density_of_the_set_}
		Since $\mathbb{A}$ is $\varepsilon$-dense in $[-B,B]$, there exists $u,v\in \mathbb{A} \cap [-B,B]$ such that $| v - 2 \varepsilon | \leq \varepsilon $ and $| u- B | \leq \varepsilon$, which implies
		\begin{align*}
			u \in& [B - \varepsilon, B]\\
			v \in& [\varepsilon, 3\varepsilon]			
		\end{align*}
		It remains to show that $\mathbb{A}(u,v,k)$ is $(3\varepsilon)^{k}$ dense in $[-(B- \varepsilon)^k, (B- \varepsilon)^k]$. We fix an $x \in [(B- \varepsilon)^{k+1},(B- \varepsilon)^{k}] $ and use the Euclidean algorithm, as follows, to find $( a_i )_{i=0}^k$ and $( b_i )_{i=0}^k$ such that  $| x - \sum_{i = 0}^{k} (u^i a_i + v^i b_i) | \leq v^k \varepsilon \leq (3 \varepsilon)^{k+1}$ and $| a_i |,| b_i | \in \mathbb{A} $, $i =0,\dots,k$. Since $ 0 \leq | \frac{x}{v^{k}} |  \leq  | \frac{(B-\varepsilon)^{k+1}}{(B- \varepsilon)^{k}}  |  \leq B$, and $\mathbb{A}$ is $\varepsilon$-dense on $[-B,B]$,  there exists a number $\tilde{a}_k \in A \cap [-B,B]$ such that 
		\begin{equation}
			\label{eq:choice_of_tilde_a_k}
		 	\biggl|\tilde{a}_k -  \biggl| \frac{x}{u^{k}}  \biggr|  \biggr| \leq \varepsilon.
		\end{equation} 
		Set $a_k = \tilde{a}_k $, if $x \geq 0$, and $a_k = - \tilde{a}_k $, otherwise. It then follows from \eqref{eq:choice_of_tilde_a_k} that  $|a_k -  \frac{x}{u^{k}}   | \leq \varepsilon$, which implies $|\frac{x - a_k u^k}{u^{k-1}}   | \leq u \varepsilon  \leq B$. Since $\tilde{a}_k \in \mathbb{A}$ and $\mathbb{A} = -\mathbb{A}$, we have $| a_k | \in \mathbb{A} $. We continue to find $a_{k-1}$. Since $| \frac{x - a_k u^k  }{u^{k-1}}| \leq B $ and by a similar way we can find an $a_{k-1}$ with $| a_{k-1} |\in \mathbb{A} $ such that $| \frac{x - a_k u^k  }{u^{k-1}} - a_{k-1} | \leq \varepsilon$, which implies $| \frac{x - a_k u^k - a_{k-1}u^{k-1} }{u^{k-2}} | \leq u \varepsilon \leq B$. Repeating the same algorithm yields the existence of  $a_i$ with $| a_i |\in \mathbb{A}$, $i = 0,\dots, k $ such that $| \frac{x - \sum_{i =0}^k a_k u^k}{u^{-1}} | \leq u \varepsilon$, which implies  $| x - \sum_{i =0}^k a_k u^k | \leq \varepsilon$. We set $y =  x - \sum_{i =0}^k a_k u^k$ and implement the Euclidean algorithm on $y$ with respect to $v$. Since $| y | \leq \varepsilon \leq B$, with a similar argument, when searching for $a_k$, there exist $b_0 \in \mathbb{R}$ such that $| b_0 | \in \mathbb{A}$ and $| y - b_0 | \leq \varepsilon$. We then get $| \frac{y - b_0}{v} | \leq  \frac{\varepsilon}{v} \leq 1 \leq B$, and, in turn, the existence of $b_1$  such that $| b_1 | \in \mathbb{A}$ and $| \frac{y - b_0}{v} - b_1  |\leq \varepsilon$, which in turn implies $| \frac{y - b_0 - b_1 v}{v^2} |\leq \frac{\varepsilon}{v} \leq B$. Repeating the same algorithm, yields the existence of $b_i \in \mathbb{R}_+$ with $| b_i  | \in \mathbb{A}$, $i =0,\dots,k$ such that  $| \frac{y - \sum_{i=0}^k v^i b_i}{v^{k+1}} | \leq \frac{\varepsilon}{v} $, which is $y - \sum_{i=0}^k v^i b_i \leq v^k \varepsilon$. It follows that
		\begin{equation*}
			\Bigl| x - \sum_{i = 0}^{k} (u^i a_i + v^i b_i) \Bigr| = \Bigl| y - \sum_{i = 0}^{k} (v^i b_i) \Bigr| \leq v^k \varepsilon \leq (3 \varepsilon)^{k+1},
		\end{equation*}
		where we used $v \leq 3 \varepsilon$, and therefore we find an element $y = \sum_{i = 0}^{k} (u^i a_i + v^i b_i)$ such that $| x - y | \leq  (3 \varepsilon)^{k+1}$. This procedure holds for all $x \in [-(B - \varepsilon)^{k+1}, (B+\varepsilon)^{k+1}]$ and therefore $\mathbb{A}(u,v,k)$ is $(3 \varepsilon)^{k} \varepsilon$-dense in $[- (B - \varepsilon)^{k+1}, (B - \varepsilon)^{k+1}]$. 


	% subsection density_of_the_set_ (end)



	% subsection representation (end)

	% \subsection{Proof of Lemma~\ref{lem:density_transfer}} % (fold)
	% \label{sub:density_on_a_subset}

	\textbf{Proof of Lemma~\ref{lem:density_transfer}}
		We first show $\mathbb{A} \cap [-C,C]$ is nonempty. As $\mathbb{A}$ is $\varepsilon$-dense in $[-B,B]$, there exists $y \in [-B,B] \cap \mathbb{A}$ such that $| y | \leq | y - 0 | \leq \varepsilon \leq C $, which concludes $y \in [-C,C] \cap \mathbb{A}$. Next, suppose, for the sake of contradiction, that there exist $x_0 \in [-C,C]$ and $y_0 \in \mathbb{A} \cap [-C,C]$ such that $| x_0 - y_0 | =  \min \{ | y - x_0  |: y \in  \mathbb{A} \cap [-C,C]  \} > 2\varepsilon$. We assume without loss of generality that $x_0 \leq y_0$. Let $x_1  = \frac{x_0 + y_0}2 \in [-C, C] \subseteq [-B,B]$. Since $\mathbb{A}$ is $\varepsilon$-dense in $[-B,B]$, there exists an $y_1 \in \mathbb{A} \cap [-B,B]$ such that $| y_1 - x_1  | \leq \varepsilon $. We have $ y_1   \leq  x_1   + | y_1 - x_1  | = y_0 - \frac{y_0 - x_0}2 + | y_1 - x_1  | < y_0 - \varepsilon + \varepsilon  = y_0 \leq C$ and $y_1 \geq x_1   - | y_1 - x_1  | = x_0 + \frac{y_0 - x_0}2 -   | y_1 - x_1  | > x_0 + \varepsilon - \varepsilon = x_0 \geq -C $, which in turn imply $y_1 \in \mathbb{A} \cap [-C,C]$. The fact that $| y_1 - x_0 | = y_1 - x_0 < y_0 - x_0 = | y_0 - x_0 | $ contradicts the definition of $y_0$. See Figure~\ref{fig:densenss} for a visualization of $y_0,y_1,x_0,x_1$.
		\begin{figure}[H]
			\centering
			\includegraphics[width=0.5\textwidth]{images/denseness.jpg}
			\caption{$y_0,y_1,x_0,x_1$}
			\label{fig:densenss}
		\end{figure}



			% Suppose $x \in [-C,C]$. We show there exists a number $y \in [-C,C] \cap \mathbb{A}$ such that $| x - y | \leq 2 \varepsilon$. Let $a_1 = \sup \{ a \in \mathbb{A} : a \leq x  \}$ and $a_2 = \{ a \in \mathbb{A} : a \geq x  \} $. We have $a_1 \leq x \leq a_2$. Since $\mathbb{A}$ is $\varepsilon$-dense in $[-B,B]$ and $x \in [-C,C] \subseteq [-B, B]$, there must be $\max \{ | x - a_1 |, | x - a_2 |   \} \leq \varepsilon$, otherwise no element in $\mathbb{A}$ can approximate $x$ up to an $\varepsilon$ error. Without loss of generality, we assume $| x - a_2 | = a_2 - x \leq \varepsilon $. 
			% \begin{enumerate}
			% 	\item If $a_2  \in [-C,C]$, then let $y = a_2 \in [-C,C] \cap \mathbb{A}$ and we have $| x - y | \leq 2 \varepsilon$.
			% 	\item If $| a_1 - x | = x - a_1 \leq 2 \varepsilon $ and $a_1 \in [-C,C]$, then let $y = a_1 \in [-C,C] \cap \mathbb{A}$ and we have $| x - y | \leq 2 \varepsilon$.
			% \end{enumerate}
			% Suppose otherwise these two cases does not hold, then either $a_1 \notin [-C,C]$  or $a_1 \in [-C,C]$ but $| a_1 - x | = x - a_1  > 2 \varepsilon$. In the first case where $a_1 \notin [-C,C]$, we have $a_1 < -C < C < a_2$, and therefore $\mathbb{A}$ can not approximate $0$, which contradicts the $\varepsilon$-denseness of $\mathbb{A}$ in $[-B,B]$.  See Fig~\ref{fig:two_impossible_cases}. In the second case, let $\hat{x} = \frac{a_1 + x}{2}$, then $| \hat{x}  - a_1  | \geq \frac{1}{2} | x - a_1 | > \varepsilon $ and $| a_2 - \hat{x} | \geq | x - \hat{x}  | > \varepsilon $, which contradicts the $\varepsilon$-denseness of $\mathbb{A}$ in $[-B,B]$. See Fig~\ref{fig:two_impossible_cases}. Overall, there must be a $y \in [-C,C] \cap \mathbb{A}$ such that $| x - y | \leq 2 \varepsilon$, and therefore $\mathbb{A}$ is $2 \varepsilon$-dense in $[-C,C]$.
			% \begin{figure}[H]
			% 	\centering
			% 	\includegraphics[width=0.5\textwidth]{images/density.jpg}
			% 	\caption{Two impossible cases}
			% 	\label{fig:two_impossible_cases}
			% \end{figure}
	% subsection density_on_a_subset (end)


	\fi
